# Supplementary material for: Multi-level Activation for Segmentation of Hierarchically-nested Classes
Source: arXiv:1804.01910 ancillary file (2018-08-21)
Supplement: Supplementary file 1 [file suppmat.pdf]

# Supplementary Material to ‘Multi-level Activation for Segmentation of Hierarchically-nested Classes’

Marie Piraud<sup>1,2</sup>, Anjany Sekuboyina<sup>1</sup>, and Björn H. Menze<sup>1</sup>

<sup>1</sup> Department of Computer Science, Technische Universität München,  
Munich, Germany,

<sup>2</sup> [marie.piraud@tum.de](mailto:marie.piraud@tum.de)

## 1 Liver lesion segmentation

We provide a second benchmark of the proposed activation function, on the dataset from the Liver Tumor Segmentation Challenge (LITS) hosted by ISBI and MICCAI in 2017. From the 130 available contrast-enhanced abdominal CT volumes, we use 85 for training, 20 for validation and 25 for testing, and further select all sagittal 2D slides which contain at least 1% of liver pixels, ending up with  $N_{\text{im}} = 10665$  training images, 2650 for validation and 3173 for testing. The images, resized to  $388 \times 388$ , are submitted to online data augmentation and fed into the U-Net-based architecture from the main text, which is trained for 80 epochs. We benchmark our proposed methods with multi-class classification, including class-reweighting in all cases due to the high class imbalance.  $\theta_2$  is selected on the validation images containing lesions and the corresponding Dice scores are reported in Fig. 1. For the test images with lesions, we report the average Dice score, and for those without lesions, we report the False Positive (FP) rate, see Table 1.

Our proposed methods converge faster and perform better than multi-class: they achieve a better Dice scores on slides containing lesions, and a lower FP rate on those without lesions. Multi-class is indeed plagued with FP in that case, in particular outside the liver. The regularization brought by multi-level activation permits to significantly reduce them, and threshold selection at validation time leads to further improvement.

## 2 Higher number of nested classes

Generalization of our method to a higher number of nested classes is obtained by adding further levels in the activation function, as in Eq. (1) of the main text, along with the corresponding thresholds. For 4 nested classes [ $\text{class-3} \subset \text{class-2} \subset \text{class-1} \subset \text{class-0}$ ], it reads

$$a(x) = \sigma [\kappa(x + h)] + \sigma [\kappa x] + \sigma [\kappa(x - h)] , \quad (1)$$

with 3 associated thresholds  $0 < \theta_1 < \theta_2 < \theta_3 < 3$ .

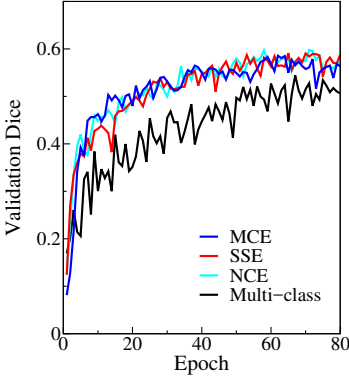

| Model           | $\theta_2$         | test Dice | FP rate |
|-----------------|--------------------|-----------|---------|
| I - Multi-class | —                  | 0.36      | 0.83    |
| II - NCE        | $\theta_2^I = 1.5$ | 0.39      | 0.73    |
| III - SSE       | $\theta_2^I = 1.5$ | 0.42      | 0.71    |
| IV - MCE        | $\theta_2^I = 4/3$ | 0.42      | 0.70    |
| V - NCE         | 1.9                | 0.46      | 0.44    |
| VI - SSE        | 1.8                | 0.46      | 0.48    |
| VII - MCE       | 1.8                | 0.45      | 0.46    |

**Fig. 1 & Table 1: Scores for liver lesion segmentation. Fig.:** Mean validation Dice scores for the methods listed in the table (rows I and V to VII). **Table:** Mean test Dice scores (slides with lesions), and False Positive rates (slides without lesions), for standard multi-class (row I) and multi-level activation (rows II-VII). In rows II to IV we use the threshold  $\theta_2^I$ . In rows V to VII,  $\theta_2$  is selected during validation and we report its mean value. Grey cells highlight significant improvement over multi-class, i.e. p-values  $< 0.05$  using the paired samples Wilcoxon test.

**Sum of Squared Error loss.** The SSE loss function is then unchanged compared to Eq. (2) of the main text.

**Modified Cross-Entropy loss.** In MCE, the pseudo-class-probabilities for each class  $c$  should peak at  $P^c(a) = 1$  for  $a = c$ , as well as go to zero at  $a = 0$  and 3. For the three-level case, this leads to the triangular structures presented in Fig. 2(a), which corresponds to

$$\begin{aligned}
 P^{c=0}(a) &= 1 - a/3, \\
 P^{c=1}(a) &= a\Theta(1-a) + (3-a)/2\Theta(a-1), \\
 P^{c=2}(a) &= a/2\Theta(2-a) + (3-a)\Theta(a-2), \\
 P^{c=3}(a) &= a/3,
 \end{aligned} \tag{2}$$

where  $\Theta(x)$  is the Heaviside function. Integrating this transformation in Eq. (4) of the main text leads to the generalized MCE loss.

**Normalized Cross-Entropy loss.** The corresponding NCE mapping is obtained when the slopes of each function is brought to one, using the softplus to prevent the gradient from becoming strictly null. It is presented in Fig. 2(b) for

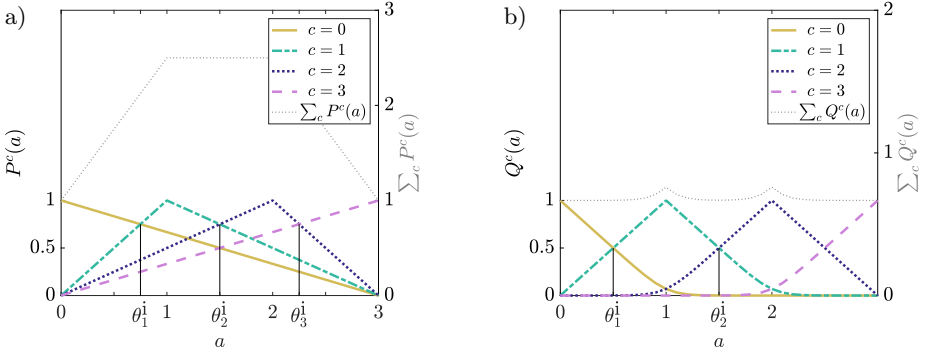

**Fig. 2:** *Class-‘probabilities’.* Functions to map the output of the activation layer  $a$  to pseudo-probabilities for four nested classes. (a)  $P^c(a)$  for the MCE loss, see Eq. (2), and (b)  $Q^c(a)$  for the NCE loss, with  $t = 10$ , see Eq. (3).

the three-level case, and reads

$$\begin{aligned} Q^{c=0}(a) &= s(1 - a), \\ Q^{c=1}(a) &= a \Theta(1 - a) + s(2 - a) \Theta(a - 1), \end{aligned} \quad (3)$$

$$\begin{aligned} Q^{c=2}(a) &= s(a - 1) \Theta(2 - a) + (3 - a) \Theta(a - 2), \\ Q^{c=2}(a) &= s(a - 2). \end{aligned} \quad (4)$$

The  $Q^c(a)$  functions, are asymptotically normalized,  $\sum_c Q^c(a) \rightarrow_{t \rightarrow \infty} 1$ , and lead to the NCE loss when integrated in Eq. (6) of the main text.

### 3 Combination with further non-nested classes

Segmentation of both nested and non-nested classes, leads to tree hierarchical structures, such as those presented Fig. 3. For those tasks, 3-class MCE and NCE can naturally be combined with standard cross-entropy, by the introduction of more output channels. We distinguish two basic situations: (i) the additional class does not have topological relation with the nested ones, as in Fig. 3(a), and (ii) the new class has a nesting relation in the intermediate class, as in Fig. 3(b). The case where the new class is nested into class-2 has been addressed in the previous section.

**Several root classes.** In the case illustrated on Fig. 3(a), the root of the tree is a standard multi-class problem without prior topological knowledge between classes 0, 1 and 2, with an additional nested class  $1b \subset 1$ . We therefore propose to use 3 output channels  $\{x_i^{(0)}, x_i^{(1)}, x_i^{(2)}\}$ . A soft-max function  $S(x_i^{(k)}) = e^{x_i^{(k)}} / \sum_{k'} e^{x_i^{(k')}}$  first permits to determine the ‘root’ class  $\{0, 1, 2\}$ , and a three-level activation on the  $\{x_i^{(1)}\}$  map is then used to segment the nested class  $1b$ . The resulting loss is the sum of the standard cross-entropy for

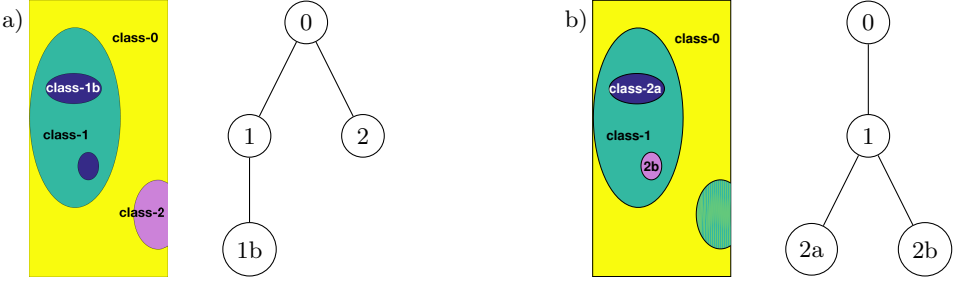

**Fig. 3:** *Combination with non-nested classes.* (a) Sketch and hierarchical tree for 4 classes with  $1b \subset 1$ . (b) Sketch and hierarchical tree for 4 classes with  $2a \subset 1$  and  $2b \subset 1$ .

maps  $\{x_i^{(0)}, x_i^{(2)}\}$ , and one of the proposed cross-entropy-based multi-level losses on map  $\{x_i^{(1)}\}$

$$\mathcal{L} = -\frac{1}{N_{\text{tot}}} \sum_{\text{pixels } i} \sum_{k \in \{0,2\}} \omega^k y_i^k \log \left( S[x_i^{(k)}] \right) + \mathcal{L}_{\text{MCE/NCE}} \left( a[x_i^{(1)} + h/2] \right). \quad (5)$$

Note that for consistency, the soft-max and the multi-level activation should be shifted with respect to each other, e.g. by using  $a(x_i^{(1)} + h/2)$  in the present case.

**Several nested classes.** Generalization of our method to the case of Fig. 3(b) can be obtained by introducing 2 output channels  $\{x_i^{(a)}, x_i^{(b)}\}$  and a multi-level activation on each of them. The loss on each channel should ignore the presence of the other nested class, such that we propose

$$\mathcal{L} = \mathcal{L}_{\text{MCE/NCE}} \left( a[x_i^{(a)}] \right) + \mathcal{L}_{\text{MCE/NCE}} \left( a[x_i^{(b)}] \right), \quad (6)$$

with the replacements  $y_i^{c=1} \rightarrow y_i^1 + y_i^{2b}$  in the first term, and  $y_i^{c=1} \rightarrow y_i^1 + y_i^{2a}$  in the second term. For inference, one then needs to devise a scheme to merge the predictions for class 1 emerging from each channel, for example by taking the union. And classes 2a and 2b are discriminated through a soft-max function in case of ambiguity.
